# Supplementary material for: SinGRAV: Learning a Generative Radiance Volume from a Single Natural Scene
Source: arXiv:2210.01202 source file (2022-10-16)
Supplement: Supplementary file 1 [file algorithm1.tex]

\RestyleAlgo{ruled}
\begin{algorithm}[hbt!]
\caption{Training process at scale $s$.}\label{alg:supp}
% \KwData{$n \geq 0$}
% \KwResult{$y = x^n$}
% \textbf{Input: $\{z_{\scale}\}_{\scale=1}^{s}$} \\
\textbf{Input:} noise volume sequence $\{z_{\scale}\}_{\scale=1}^{s}$ \\ 
\textbf{Output:} generated volume $\tilde{V}_{s}$, rendered image $\tilde{x}_{\scale}$ and depth $\tilde{d}_{\scale}$ \\
\textbf{Parameters:} parameters in $G_{s}$ and $D_{s}$ \\
\While{$i<T$}
{
    \eIf{$i<T_1$}
    {
        optimize $G_s$ with $\loss_{rec}$ according to $\loss_{rec}$ Eq.(\ref{eq:loss_rec});
    }
    {
    \eIf{$J<D_{steps}$}{
       $\tilde{V}_s = \{G_{\scale}\}_{\scale=1}^{s}(\{z_{\scale}\}_{\scale=1}^{s},e_1)$;\\
       $\tilde{x}_s=\pi(\tilde{V}_s)$;
    }{
    }
        optimize $G_s$ and $D_s$ according to the loss given in Eq. (\ref{eq:loss_total});
    }
}
% $y \gets 1$\;
% $X \gets x$\;
% $N \gets n$\;
% \While{$N \neq 0$}{
%   \eIf{$N$ is even}{
%     $X \gets X \times X$\;
%     $N \gets \frac{N}{2} $ \Comment*[r]{This is a comment}
%   }{\If{$N$ is odd}{
%       $y \gets y \times X$\;
%       $N \gets N - 1$\;
%     }
%   }
% }
\end{algorithm}
